# Supplementary material for: Bayesian inference of wall torques for active Brownian particles
Source: arXiv:2409.03533 source file (2024-09-05)
Supplement: Supplementary file 1 [file supplements.pdf]

# Supplementary Information for "Bayesian inference of wall torques for active Brownian particles"

S. Lambert

M. Duchêne

S. Klumpp

September 5, 2024

## 1 Least-squares Fit

### 1.1 Varying number of test sites

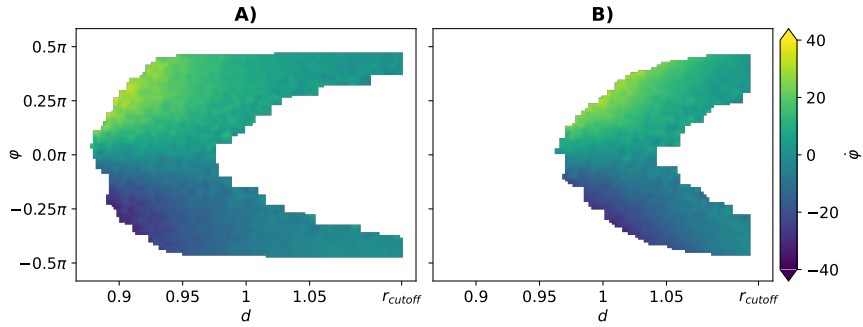

Figure 1: Torque data from R-type simulations for number of test sites  $N_S = 2$  in **A)** and  $N_S = 400$  in **B)** as a function of the distance  $d$  from the wall and orientation  $\varphi$  to the wall.

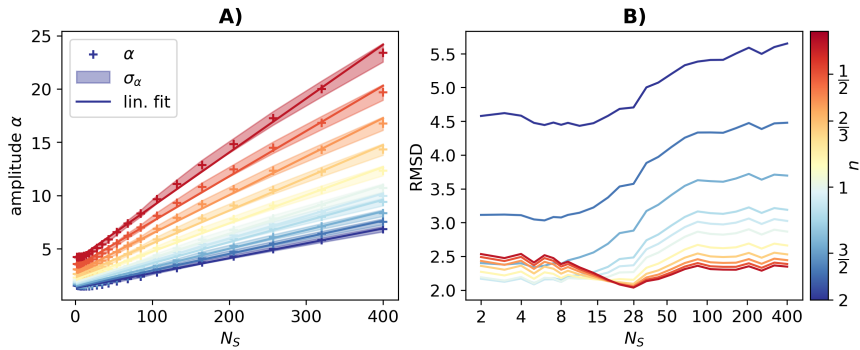

Figure 2: Optimal  $\alpha$  values as a function of number of test sites,  $N_S$ , representing the rod-like particle. **A)** Fitted amplitudes for a single-mode torque function. A linear relation between the torque strength and the number of nodes can be observed. This is expected as the equidistantly distributed test sites each produce their own unadjusted torque. **B)** Root mean square deviation (RMSD) of the fit. Minimization of this quantity is the optimization objective. Short periods show a significantly worse performance. The optimal performance depends on the number of test sites used.

## 1.2 Varying Peclet number

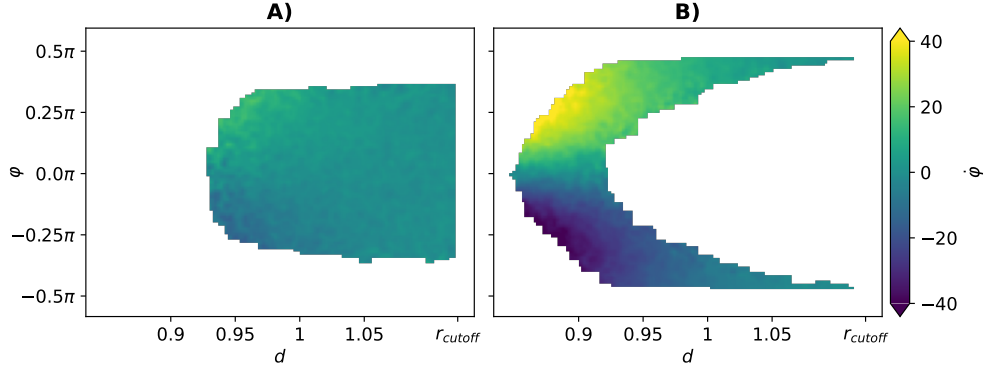

Figure 3: Torque data from R-type simulations for Péclet numbers  $Pe = 10$  in **A)** and  $Pe = 200$  in **B)** as a function of the distance  $d$  from the wall and orientation  $\varphi$  to the wall.

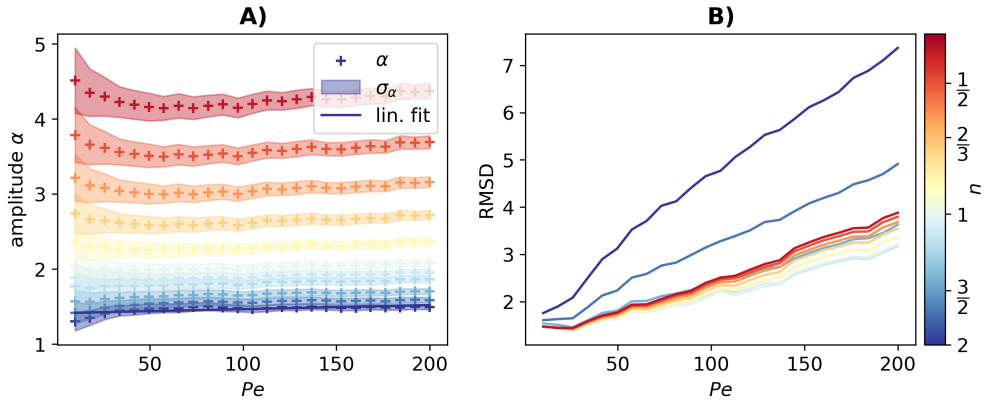

Figure 4: Dependence of the fit on the Péclet number: **A)** Optimized torque parameters  $\alpha$  for a single-mode torque function  $f$ . The parameter is largely independent of the particle's activity. For low activities, the 68% confidence intervals are wider. **B)** RMSD of the fits. Highly oscillatory torque functions perform significantly worse than low oscillatory torque functions.

### 1.3 Varying WCA strength

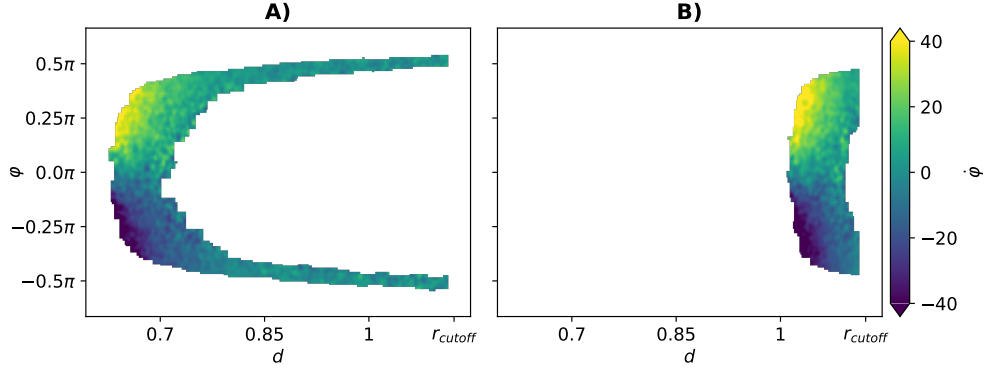

Figure 5: Torque data from R-type simulations for different wall-force parameters of  $\varepsilon = 0.1$  in **A)** and  $\varepsilon = 50$  in **B)** as a function of the distance  $d$  from the wall and orientation  $\varphi$ .

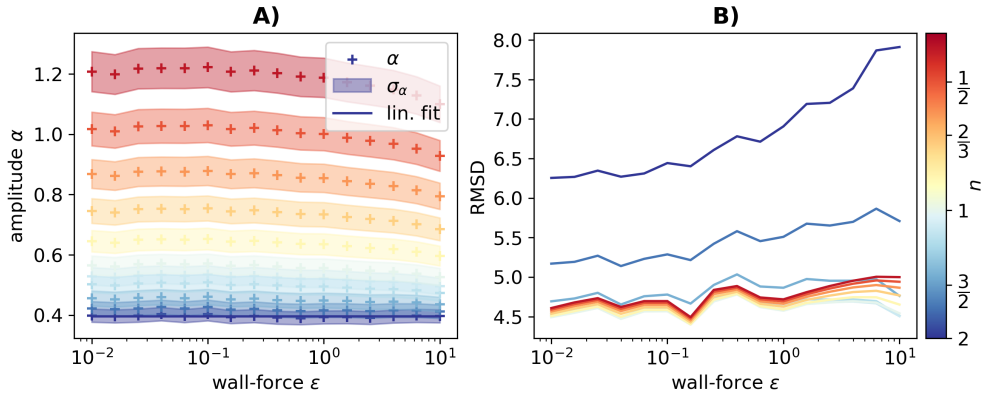

Figure 6: Dependence of the fit on the wall-force parameter  $\varepsilon$ : **A)** Fitted amplitudes  $\alpha$  as a function of the wall-force parameter  $\varepsilon$  for different periods  $n$ . The amplitude stays approximately constant. **B)** The RMSD of the predicted data slightly increases for higher wall forces. This might occur because the "tails" of the binned data with respect to the distance of the wall  $x$  do not occur for high wall forces, which can be seen in figure 5.

## 1.4 Multimode Fit

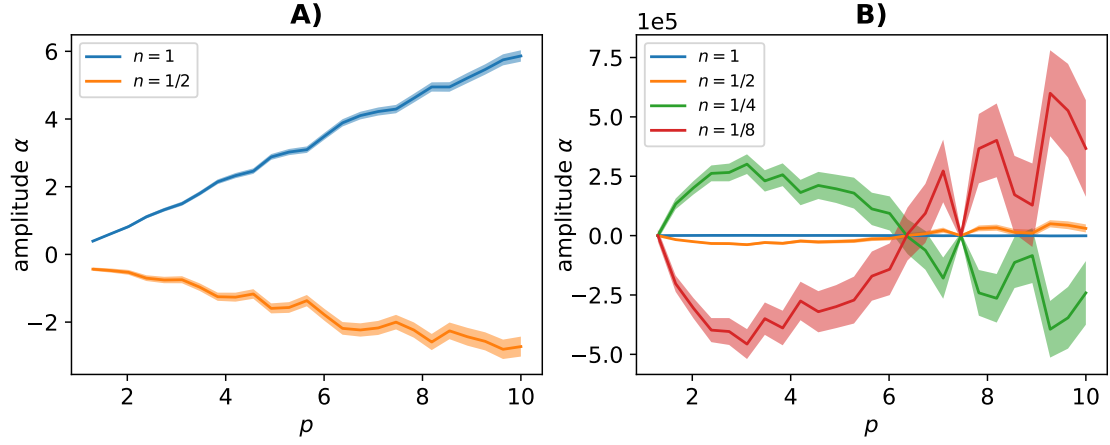

Figure 7: Fit of torque data from R-type simulation with two (A) and four (B) modes simultaneously. While 2 modes show a stable ratio of  $\alpha_1$  and  $\alpha_2$  (with opposite sign) for all aspect ratios  $p$ , for four modes, the fit composes torque for short and long rods with opposite signs for the higher frequency components.

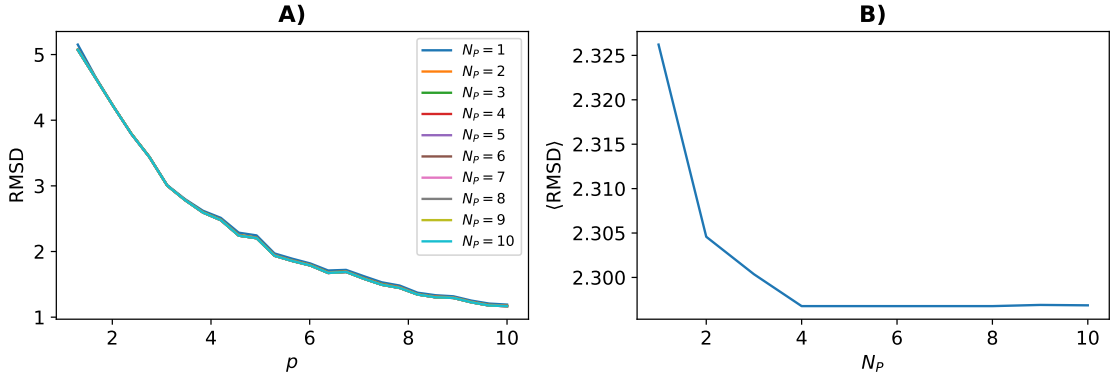

Figure 8: Performance of the fitting procedure for different numbers of modes,  $N_p$ , that compose  $f$ . A) RMSD as a function of the aspect ratio  $p$ , varying  $N_p$ . There is no significant difference in fit performance due to including higher orders. B) The same data averaged over all aspect ratios  $p$ . For small aspect ratios, the RMSD is up to 1% worse when using a single mode than four or more modes.

## 2 Bayesian Inference

### 2.1 Assimilation / State Estimation

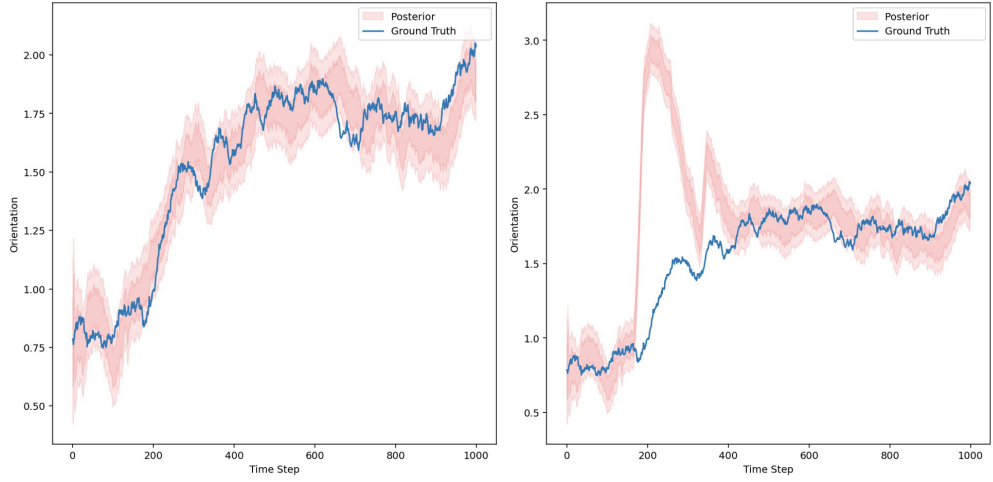

Figure 9: Filtering of the orientation  $\varphi$ . The red bands denote the 68% and 95% high-density interval (HDI) of the posterior distribution of the ABP orientation. The blue line is the ground truth from the actual simulation. Left: filtering using the ground truth parameters, Right: filtering using 10x the ground truth parameters, resulting in higher torques  $f$  than in the actual simulation. The filter closely follows the true dynamics when using the ground truth parameters. In contrast, when using the wrong parameters, there will be a significant gap between the posterior distribution of  $\varphi$  and the truth. The inference penalizes the discrepancy, as the ground truth is highly unlikely under the wrong parameters, leading to a lower posterior density.

## 2.2 Comparison of Kalman Filter with Particle Filter

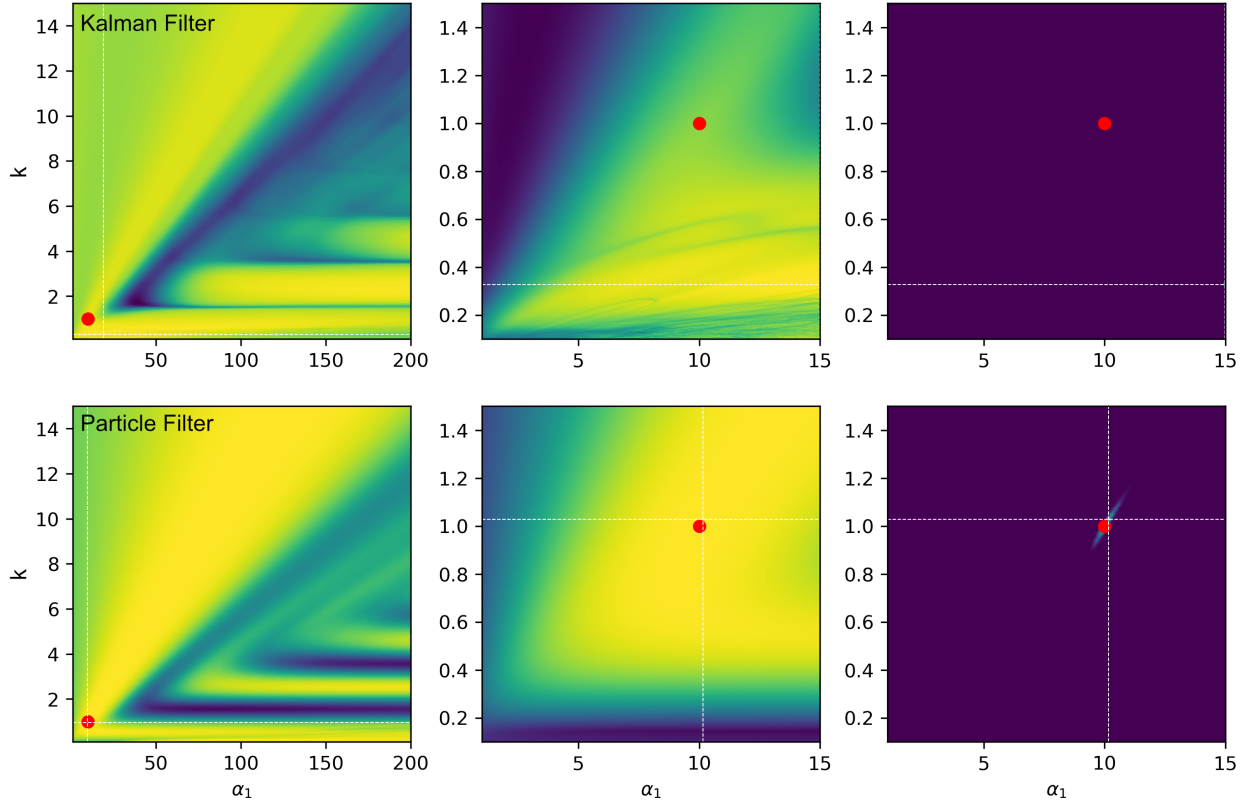

Figure 10: Comparison between the Kalman filter and the particle filter. Inference is done using a single-mode torque model, with amplitude  $\alpha_1$  and frequency  $k = 1/n$ . The top row shows the results using a Kalman filter, and the bottom row uses a particle filter. The first two columns are drawn with a logarithmic color scale to visualize the complex structure of the posterior; the third column is drawn linearly. The red dot denotes the ground truth used in ABP (type-A) simulations. The white dashed line indicates the mode of the distribution. The particle filter gives an unbiased estimate of the posterior, albeit at a much increased computational cost compared to the Kalman filter. The Kalman filter recovers qualitative features of the posterior but fails to recover the ground truth. In particular, the estimation features a fractal region for low  $k$  and high  $\alpha_1$ . We attribute this to the instability of the Kalman filter due to large torques and strong oscillations in these regions.

## 2.3 Envelope Fitting

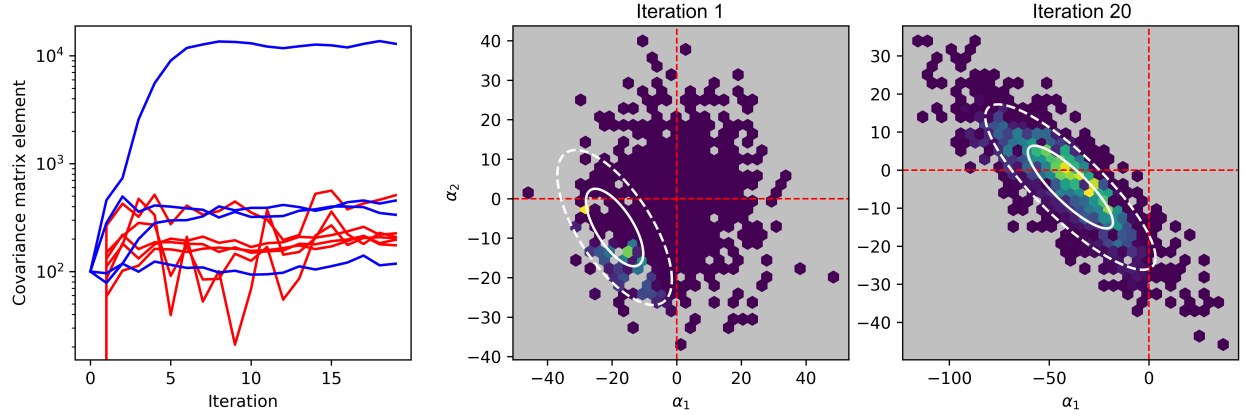

Figure 11: Fitting of the Gaussian envelope to the posterior distribution. The evolution of the entries of the covariance matrix is depicted on the left. Blue lines are the diagonal entries, and red lines are the off-diagonals. The center depicts the first iteration of the fitting procedure. The parameter space is splattered with samples around the initial guess, indicated with red dashed lines. A Gaussian is fitted to the detected posterior mass, indicated by white ellipses for one and two standard deviations. The new distribution is used as a base for the next search. After enough iterations, the envelope stabilizes around the posterior high-density region. It can then be used as an approximation to the posterior or a proposal distribution for MCMC sampling.

## 2.4 Varying amount of data used for inference

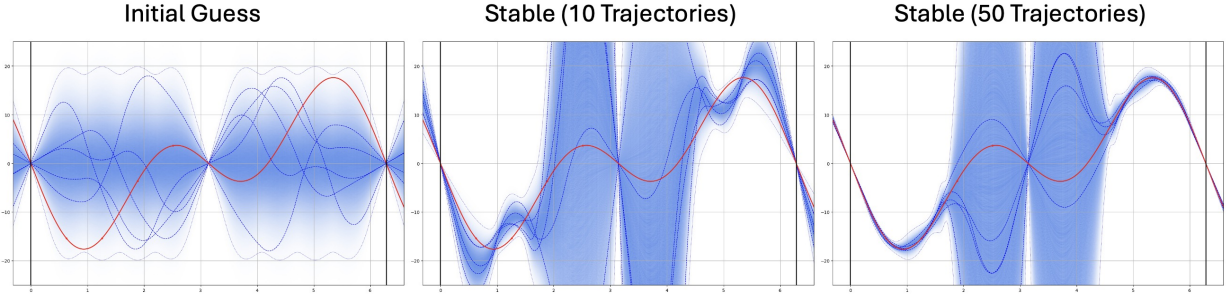

Figure 12: Inference of an ABP's torque function  $f$  (represented by B-splines). This serves as a test case for the procedure, as we know the exact  $f$  used. The red curve shows the ground truth torque used for the ABP simulations. A) The envelope to the posterior is initialized to a correlation-free multivariate Gaussian. A fitting procedure is applied to bring the Gaussian closer to the true posterior given B) 10 and C) 50 trajectories. After convergence, we can sample from the posterior. Blue dashed lines showcase individual samples, and the overall density of the posterior is shaded blue. The torque function is learned well in regions that are consequential to the system's actual dynamics. This primarily includes the inbound direction to the wall, where the HDI closely wraps the ground truth torque. Orientations facing away from the wall are not learned well, as indicated by the wide HDI.
